# Supplementary material for: A light induced metastable magnetic texture uncovered by in-situ Lorentz microscopy
Source: arXiv:1609.04000 ancillary file (2016-09-13)
Supplement: Supplementary file 1 [file supplement.pdf]

# Supplement Material - A light induced metastable magnetic texture uncovered by in-situ Lorentz microscopy

Tim Eggebrecht,[†,§] Marcel Möller,[‡,§] J. Gregor Gatzmann,[‡] Nara Rubiano da Silva,[‡] Armin Feist,[‡] Ulrike Martens,[¶] Henning Ulrichs,[†] Markus Münzenberg,[¶] Claus Ropers,[‡] and Sascha Schäfer[*,‡]

†*I. Physical Institute, Georg-August-University, Göttingen, Germany*

‡*IV. Physical Institute, Georg-August-University, Göttingen, Germany*

¶*Interface and Surface Physics, Ernst-Moritz-Arndt-University, Greifswald, Germany*

§*These authors contributed equally to this work.*

E-mail: schaefer@ph4.physik.uni-goettingen.de

## Thermal transient after optical excitation

For a more detailed discussion of the microscopic origins leading to the glass formation, we consider the transient thermal state of the iron/silicon nitride bilayer after optical excitation (cf. Fig. 1(b)). With silicon nitride being transparent at the employed wavelength, the optical pulse energy is first deposited in the iron thin film, leading to an ultrafast rise of the electron temperature, subsequently equilibrating with the spin and lattice system on a time scale below 1 ps.[1–3] In the picosecond regime considered here, we describe the thermal state of the iron film by a single-temperature model with a maximum of the temperature transient, which exceeds the Curie temperature $T_{\mathrm{C}} = 1041\,\mathrm{K}$ at high laser fluences, resulting

in heating rates of up to $10^{15}$ K/s. We note that for high fluences the temperature approaches $T_\mathrm{C}$ (Fig. 1(b)), and a critical regime is reached. For such conditions, the temperature response of the spin system is slowed down,[4] so that the typical non-thermal peak in spin temperature observed in ultrafast optical studies is expected to be largely damped.

On longer timescales (∼100 ps), the iron overlayer is cooled down by the underlying silicon nitride membrane, which is optically transparent at the employed wavelength. For example, for an optical fluence of 10 mJ/cm$^2$, we estimate that the iron layer is initially heated to a peak temperature of 1265 K. Taking into account the relative heat capacities of the iron and silicon nitride layer, and the thermal boundary resistance[5] between the two layers, a 330 K temperature decrease after local film-substrate equilibration is obtained, with a cooling rate larger than $10^{12}$ K/s. On longer timescales, slow lateral heat transport across the membrane area ultimately brings the bilayer system back to room temperature. Within this simple thermal model, we expect that the peak iron temperature exceeds $T_\mathrm{C}$ at an optical fluences of about 7.5 mJ/cm$^2$, in reasonable agreement with the experimentally observed fluence threshold of 11.5 mJ/cm$^2$ for vortex-antivortex generation. The difference in both values might be attributed to the specific optical properties of the polycrystalline iron film, as well as potential ultrafast electronic couplings[6] between the iron and silicon-nitride layer.

## Lorentz microscopy and magnetization reconstruction

The Lorentz micrographs reported in the main text were obtained in a JEOL 2010F and a JEOL 2100F transmission electron microscope, using a low magnification imaging mode, in which the main objective lens is turned off. In this setting, the magnetic field at the sample position is reduced to about 190 Oe.[7,8] For increased magnetic background fields (with the objective lens partially turned on), we observed that vortex-antivortex networks can be annihilated at lower laser fluences, compared to annihilation without applied field.

With the full magnetic field of the main objective lens (about 2 T) applied to the sample, the vortex network vanishes. Later experiments were conducted in a modified microscope with a dedicated Lorentz objective lens, in which the sample is located within a permalloy shield (residual magnetic field below 5 Oe,[8] and comparable vortex-antivortex networks were generated.

We reconstruct the in-plane magnetization of the sample from the image contrast in the Lorentz micrographs, employing a *transport-of-intensity equation* (TIE) approach.[9] TIE allows for a reconstruction of the spatial phase distribution $\Phi(\boldsymbol{r})$ imprinted on the imaging electron wave front by utilizing a through-focus image series $I(\boldsymbol{r}, z)$ :

$$\boldsymbol{\nabla}\left[I(\boldsymbol{r},0)\boldsymbol{\nabla}\Phi(\boldsymbol{r})\right] = -\frac{2\pi}{\lambda}\frac{\partial I(\boldsymbol{r},z)}{\partial z}\bigg|_{z=0}, \tag{S1}$$

where $\boldsymbol{r}$ is the position in the $x$-$y$ (sample) plane, $z$ the defocus of the Lorentz image and $\lambda$ the electron wavelength.

Following Eq. (S1), the phase can be written as

$$\Phi(\boldsymbol{r}) = C' \sum_{i=1}^{2} \mathcal{F}^{-1}\left[\frac{q_i}{|\boldsymbol{q}|^2}\right] * \left(\frac{\mathcal{F}^{-1}\left[\frac{q_i}{|\boldsymbol{q}|^2}\right] * \frac{\partial I(\boldsymbol{r},z)}{\partial z}\Big|_{z=0}}{I(\boldsymbol{r},0)}\right), \tag{S2}$$

where $C'$ is a constant, $\mathcal{F}$ represents the two-dimensional spatial Fourier transform in the sample plane, and $\boldsymbol{q} = q_1\boldsymbol{e}_1 + q_2\boldsymbol{e}_2$ is the reciprocal space coordinate. For the smooth nanocrystalline sample employed here, in-focus conditions result in electron micrographs with a constant image intensity, so that $I(\boldsymbol{r}, 0) = I_0$, as shown in Fig. S1(b). Therefore, different from the imaging of magnetic nanostructures,[10,11] the change of image intensities with defocus can be already be deduced from a single out-of-focus image (Fig. S1(a,c)), and no alignment with an in-focus or several out-of-focus images is required.

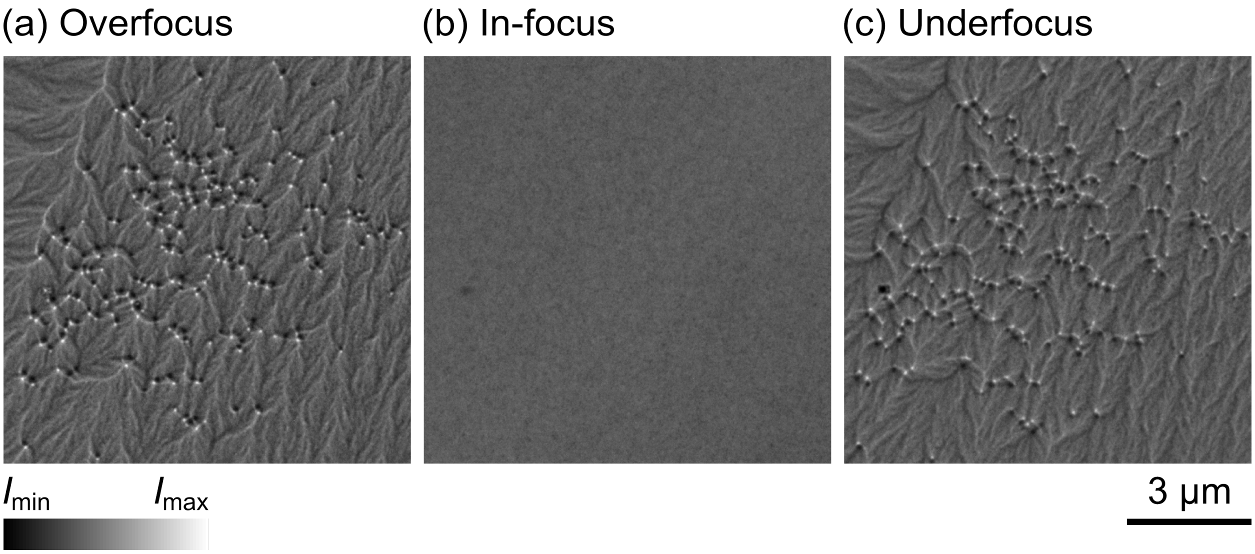


Figure S1: Electron micrographs of an iron/silicon nitride bilayer with a vortex-antivortex network recorded in **(a)** overfocus, **(b)** in-focus and **(c)** underfocus conditions. Due to the smooth surface in-focus condition exhibit no contrast, while **(a)** and **(c)** yield inverse contrast. For ease of comparison, the image magnification and orientation of **(b)** and **(c)** and was adjusted to match **(c)**.

Using the convolution theorem $f * g = \mathcal{F}^{-1}\left[\mathcal{F}\left[f\right] \cdot \mathcal{F}\left[g\right]\right]$, we obtain

$$\Phi(\boldsymbol{r}) = \frac{C'}{I_0}\mathcal{F}^{-1}\left[\frac{\mathcal{F}\left[\left.\frac{\partial I(\boldsymbol{r},z)}{\partial z}\right|_{z=0}\right]}{|\boldsymbol{q}|^2}\right]. \tag{S3}$$

For small defocus values $\Delta z$, the longitudinal derivative of the image intensity can be approximated by

$$\left.\frac{\partial I(\boldsymbol{r},z)}{\partial z}\right|_{z=0} \approx \frac{I(\boldsymbol{r},\Delta z) - I(\boldsymbol{r},0)}{\Delta z} = \frac{I(\boldsymbol{r},\Delta z) - I_0}{\Delta z}, \tag{S4}$$

so that $\partial I(\boldsymbol{r},z)/\partial z$ is directly proportional to the image contrast. To avoid amplification of low-frequency noise in applying Eq. (S3), we adopt a Tikhonov-like regularization scheme,[12] calculating the phase from

$$\Phi(\boldsymbol{r}) = C\mathcal{F}^{-1}\left[\frac{\mathcal{F}\left[I(\boldsymbol{r},\Delta z) - I_0\right]}{|\boldsymbol{q}|^2 + |\mathrm{d}\boldsymbol{q}|^2}\right], \tag{S5}$$

with a small regularization constant $|\mathrm{d}\boldsymbol{q}|$, which was fixed at $2.47\,\mu\mathrm{m}^{-1}$. Truncation artifacts in the numerical Fourier transform of the Lorentz micrograph are minimzed by utilizing an image symmetrization scheme.[13] As a consistency check, we use the reconstructed phase and calculate the Lorentz contrast using Eq. (S1), indeed, obtaining a faithful representation of the original electron micrographs, as shown in Fig. S2.

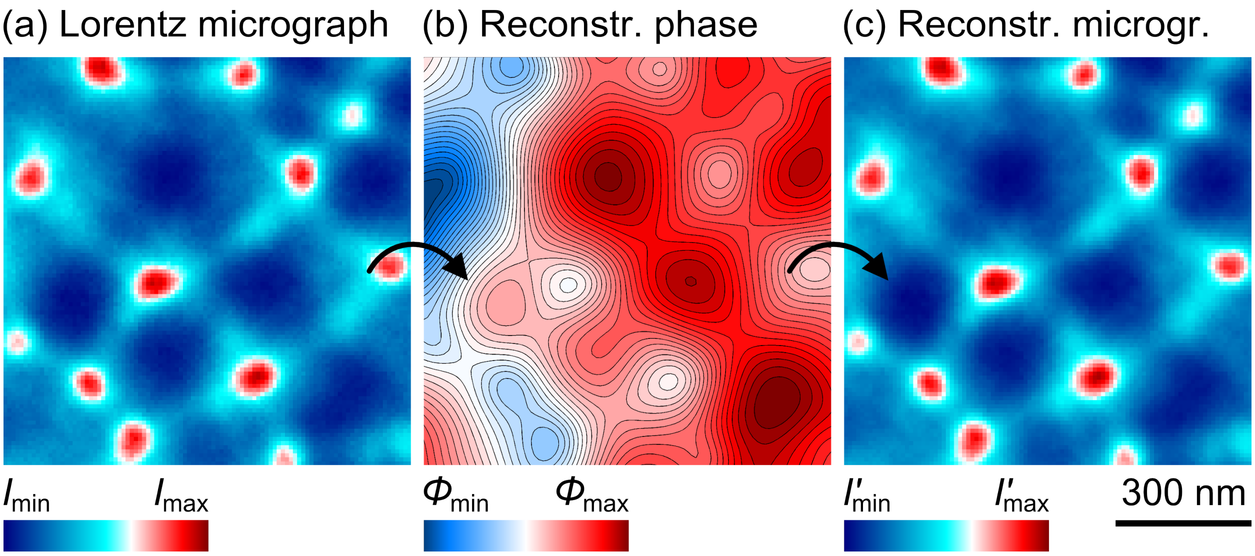


Figure S2: **(a,b)** Lorentz micrograph (a) and corresponding transmitted electron phase (b) obtained by a TIE approach. **(c)** For a sufficiently small value of the regularization constant ($|\mathrm{d}\boldsymbol{q}| = 2.47\,\mu\mathrm{m}^{-1}$), the reconstructed real space image (obtained from the phase in (b) together with Eq. (S1)) is in close agreement with the original Lorentz image.

Finally, from the gradient of the reconstructed phase $\Phi(\boldsymbol{r})$, we determine the local in-plane magnetization:

$$\boldsymbol{\nabla}\Phi(\boldsymbol{r}) = -\frac{\mathrm{e}}{\hbar}\left[\boldsymbol{B}(\boldsymbol{r}) \times \boldsymbol{n}\right] t(\boldsymbol{r}). \tag{S6}$$

Here, $\boldsymbol{B}(\boldsymbol{r})$ is the local magnetic induction of the film (including fringing fields), $\boldsymbol{n}$ the unit normal in beam direction and $t(\boldsymbol{r})$ the local film thickness. To demonstrate that the spatial phase variation is caused by the magnetic texture of the sample, we additionally recorded an Lorentz micrograph with the sample turned upside down. As shown in Fig. S3, image contrast is reversed in the rotated sample, as expected from Eq. (S6). Electrostatic contribution, visible at a dust grain indicated in Fig. S3, show no contrast change.

For the calculation of the experimental defect pair correlation function, we consider the Hessian matrix of the phase surface. We find that the position of the maxima and minima of its determinant are in close agreement with extrema and saddle points of the intensity in the Lorentz micrographs.

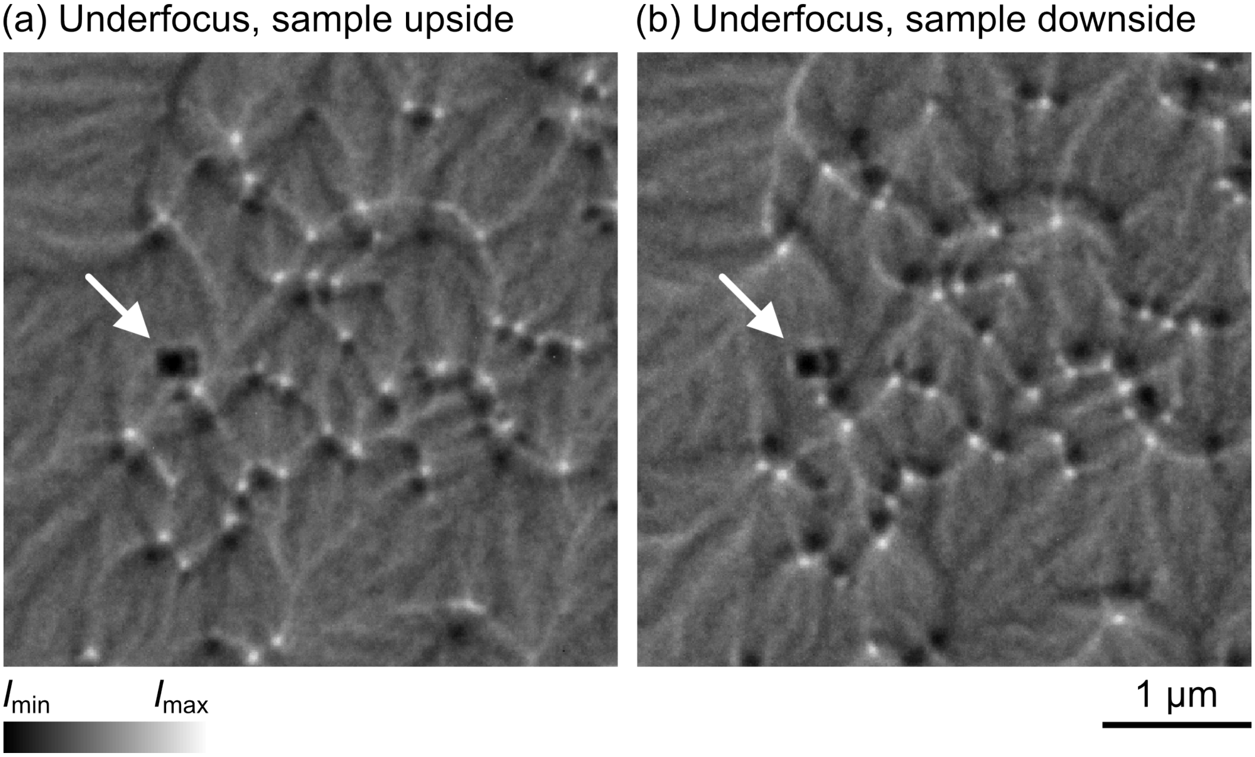


Figure S3: Contrast reversal upon sample rotation **(a)** Enlarged section of the micrograph shown in Fig. S1(c). **(b)** has the same defocus level but with a flipped sample (for better comparison this image is mirrored). The contrast of the vortex-antivortex network invertes upon sample rotation, verifying its magnetic origin, whereas the contrast of a dust grain (indicated by arrow) shows no change.

# Optical excitation below fluence threshold

In the main article, we discuss the effect of high-intensity laser pulses on thin polycrystalline iron films, yielding dense vortex networks above a well-defined laser fluence. Below this fluence threshold, the magnetic ripple structure persists after optical excitation, but with local domain rearrangements, as shown in Fig. S4. We found that such optically induced changes

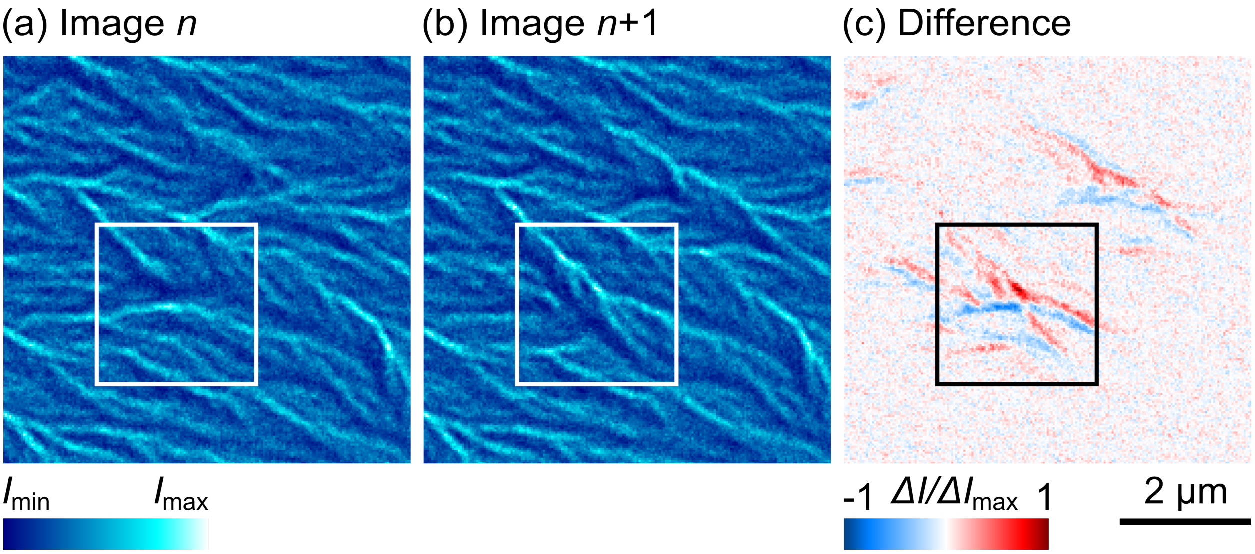


Figure S4: **(a,b)** Lorentz micrographs of the iron film before and after optical excitation, respectively, with an optical fluence below the threshold for vortex generation. Local changes in the magnetic ripple structure are observed (marked by rectangle), further highlighted in the image difference shown in **(c)**.

in the domain configuration often occur at bifurcating domain walls triggering extended magnetization changes on micrometer length scales. Subsequent laser pulses regularly lead to alternating transitions between bistable domain configurations.

For a quantitative statistical analysis of both the optically induced magnetization changes within the ripple structure and the vortex-antivortex network, we analyzed correlations between sequential Lorentz micrographs within a larger image data set (number of images $N = 100$). Between subsequent images, a single optical laser pulse was applied. First, we considered the squared intensity differences

$$D(\boldsymbol{r}) = \sum_{n=1}^{N-1} \frac{\Delta I_n(\boldsymbol{r})^2}{N-1}, \tag{S7}$$

where $\Delta I_n(\boldsymbol{r})$ is the difference between adjacent images. Fig. S5(a,b) displays the difference map $D(\boldsymbol{r})$ for below- and above-threshold optical excitation, respectively. Below threshold (Fig. S5(a)), local maxima are observed in the difference map, indicating regions with an unstable magnetic configuration, easily switchable by optical excitation. Above threshold

(Fig. S5(b)), the position of newly generated vortices is not correlated to the configuration of the original ripple structure, resulting in a largely homogeneous difference map. We note that, for the polycrystalline film studied here, film granularity may lead to vortex pinning with typical nanoscale distances between pinning sites.[14] However the average grain size in the iron thin films is smaller by one order of magnitude compared to the typical magnetic defect distances. Furthermore, we observe no preferential vortex locations when averaging over a large number of images from laser-induced networks.

Finally, we evaluate the Pearson product-moment correlation coefficient $C(\boldsymbol{r}_1, \boldsymbol{r}_2)$ between optically induced intensity changes at image pixels $\boldsymbol{r}_1$ and $\boldsymbol{r}_2$:

$$C(\boldsymbol{r}_1, \boldsymbol{r}_2) = \frac{\sum_{n=1}^{N-1} \Delta I_n(\boldsymbol{r}_1) \Delta I_n(\boldsymbol{r}_2)}{\sqrt{\sum_{n=1}^{N-1} \Delta I_n(\boldsymbol{r}_1)^2} \sqrt{\sum_{n=1}^{N-1} \Delta I_n(\boldsymbol{r}_2)^2}}. \quad \text{(S8)}$$

In Fig. S5(c,d), we plot the correlation coefficient $C(\boldsymbol{r}_1, \boldsymbol{r}_2)$ depending on $\boldsymbol{r}_2$ for fixed reference pixels $\boldsymbol{r}_1$ (indicated by crosshairs). Low-fluence optical excitation leads to long-range correlated magnetic changes recurring over many excitation cycles (Fig. S5(c)). In contrast, subsequent Lorentz images of newly formed vortex networks, exhibits no long-range order, as expected from the analysis of defect pair-correlation functions in the main text.

# Simulation of a quenched vortex state within a simple two-dimensional XY model

To illustrate the processes which are involved in the optically induced generation of a vortex glass, we calculate the quenching behavior of the classical two-dimensional (2D) XY model.[15] Specifically, we consider a system of classical in-plane oriented spins arranged on a two-dimensional lattice. The Hamiltonian of this model can be written as

$$H = -J \sum_{\langle i,j \rangle} \cos(\theta_{ij}), \quad \text{(S9)}$$

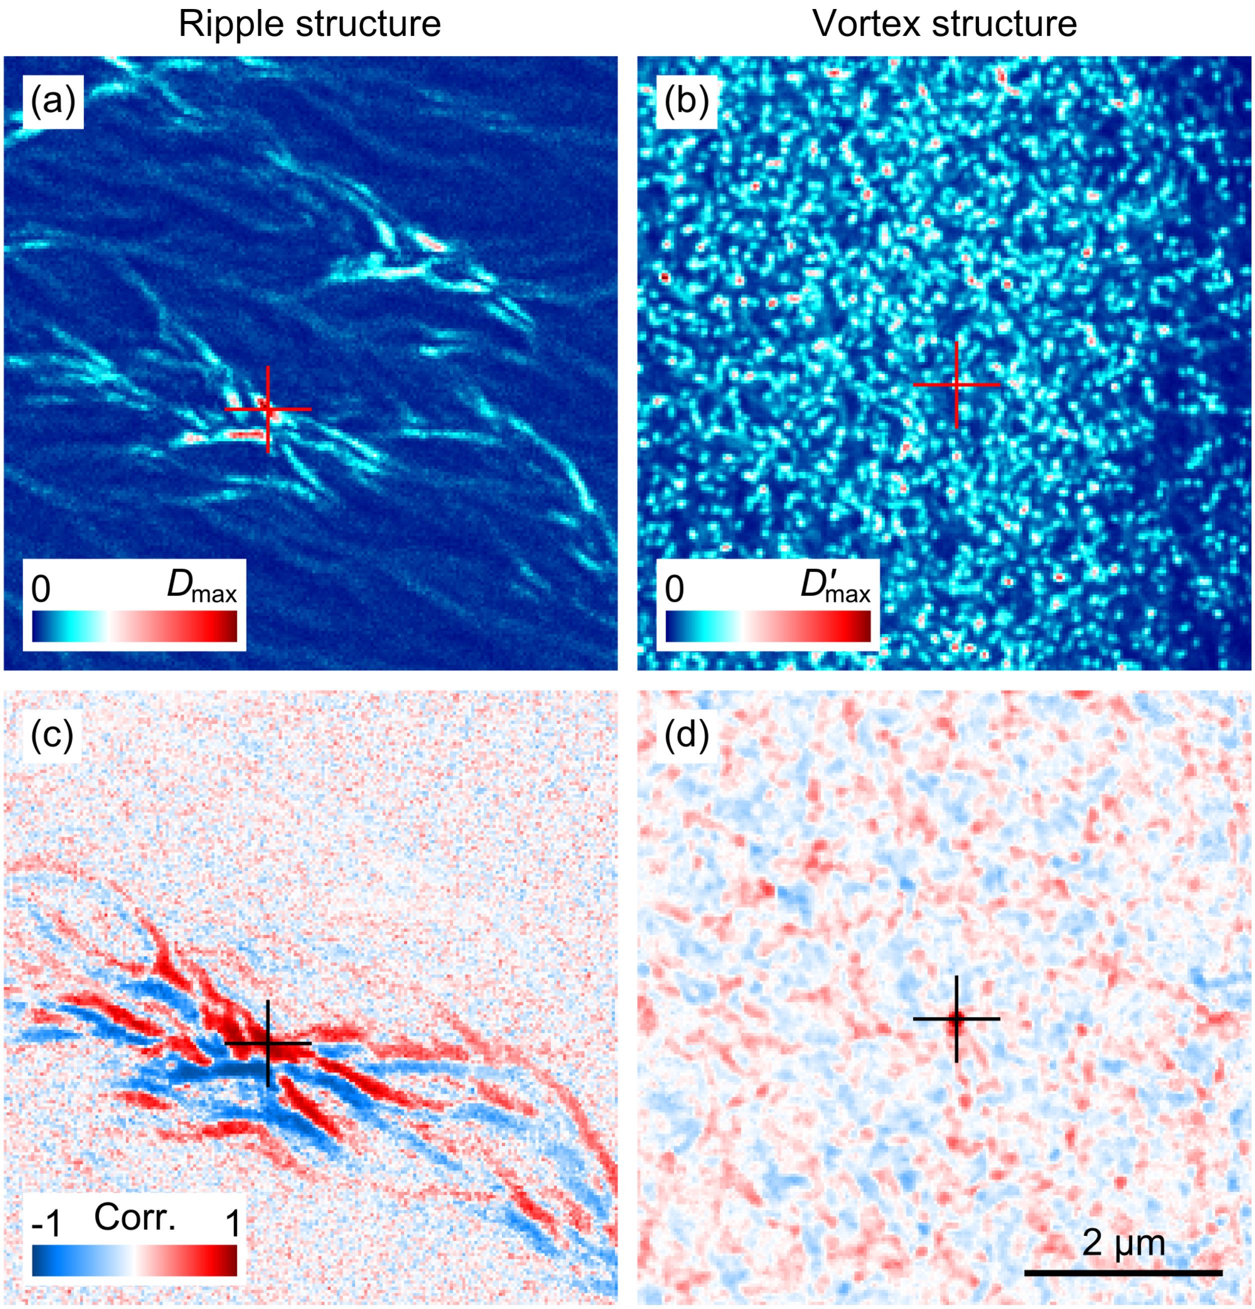


Figure S5: Statistical analysis of the optically induced magnetization changes for the sample region shown in Fig. S4. Summed square differences **(a,b)** and spatial correlation coefficients **(c,d)** are evaluated for excitation below and above threshold, respectively. Crosshair indicates the fixed reference point for the evaluation of the correlation coefficient (see text).

where $\theta_{ij}$ is the angle between the direction of the ith and jth spin, $\langle i,j \rangle$ is the sum over all nearest-neighbors, and $J$ the coupling constant between adjacent spins. For our calculations, we chose a quadratic spin lattice consisting of $100 \times 100$ sites with periodic boundary conditions and adopt a reduced temperature scale $T_{\mathrm{r}} = k_{\mathrm{B}}T/J$ ($k_{\mathrm{B}}$: Boltzmann constant, $T$: temperature). In equilibrium, the 2D XY model unsydergoes a Berezinskii-Kosterlitz-Thouless phase transitions[16,17] at a finite temperature $T_{\mathrm{KT}}$), without breaking a continuous symmetry. At the phase transition, spatial spin correlations change from a power-law dependence (low temperature phase) to an exponentially decaying behavior (high temperature phase), driven by the dissociation of vortex-antivortex pairs.[16] Out-of-equilibrium dynamics of the 2D XY model have been extensively investigated, including its response to instantaneous and linear temperature quenches.[18,19] Here, we calculate the number of remaining vortices and antivortices after a rapid exponential quench across the phase transition, using the Metropolis Monte Carlo method.[20] We start with a system of aligned spins, which we equilibrate for $3 \cdot 10^6$ Monte Carlo steps (MC) at an elevated temperature $T_{\mathrm{r,max}}$, followed by an exponential quench with a decay time of $\tau = 10^6$ MC, asymptotically reaching a reduced temperature of $T_{\mathrm{r}} = 0$. In the course of the simulation, we keep track of the number of vortices and antivortices by calculating the local winding number $w$ around each lattice site (Fig. S6 (a,b)). In addition, we extracted the radial pair correlation functions from the simulated spin lattice (Fig. S6(c)) which closely resemblances the measured results presented in Fig. 3(d) of the main text. We note that in the simulation the graph for vortex-antivortex and vortices correlations (red and blue curve) are independent of the vortex curling direction.

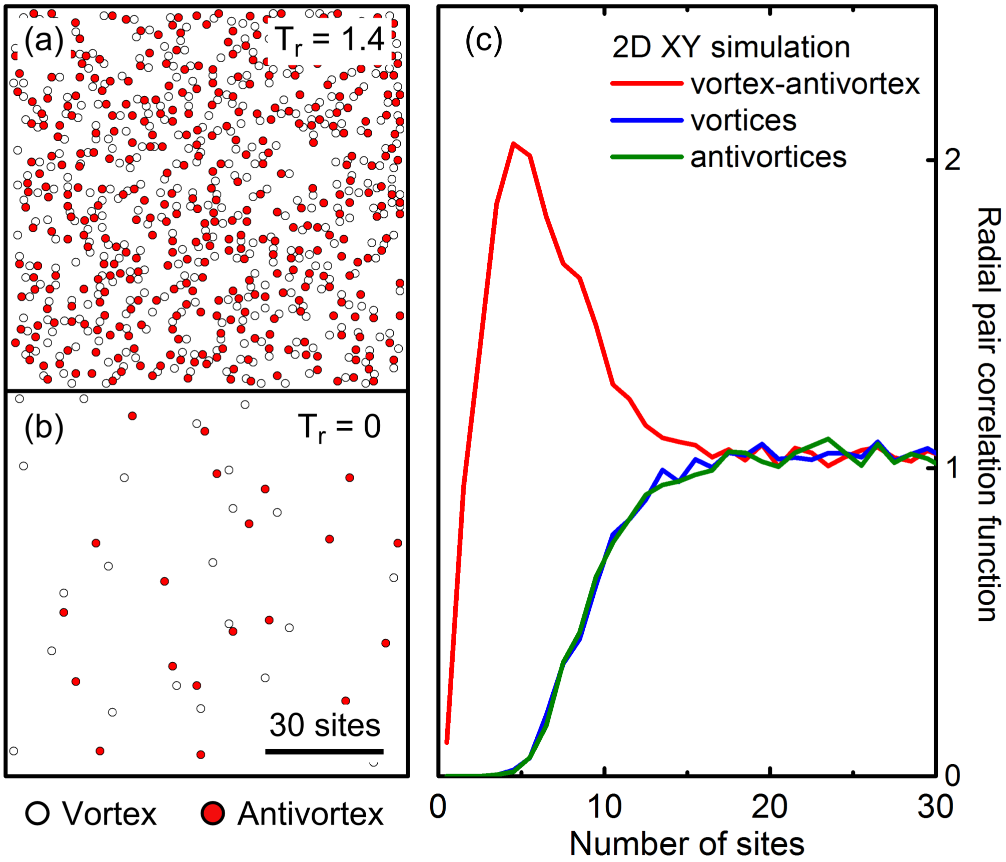


Figure S6: Quench-induced defects in a 2D spin lattice. **(a,b)** Snapshots of MC simulation during a spin quench, taken at the initial temperature $T_\mathrm{r} = 1.4$ **(a)** and the final state at $T_\mathrm{r} = 0$. **(c)** Extracted radial pair correlation function for quenched state averaged over 800 MC runs.

# Movie captions

- Movie S1: Light-induced magnetic phase. Single laser pulses at a fluence of $F = 13.1\,\mathrm{mJ/cm^2}$ generate metastable vortex phase within the central part of the optical focal spot. Between high-intensity optical pulses, the magnetic ripple structure was recovered, by applying sub-threshold optical pulses.
- Movie S2: Sub-threshold optical excitation. Optical pulses with a fluence of $F = 8.9\,\mathrm{mJ/cm^2}$ induce local changes in the equilibrium ripple structure, with no generation of magnetic vortices.
- Movie S3: Network annihilation process. After initial excitation with a single optical pulse at a fluence of $F = 12.7\,\mathrm{mJ/cm^2}$, subsequent low-fluence pulses ($F = 10.8\,\mathrm{mJ/cm^2}$) relax the sample to its equilibrium ripple structure.

# References


(1) Kampfrath, T.; Ulbrich, R. G.; Leuenberger, F.; Münzenberg, M.; Sass, B.; Felsch, W. *Phys. Rev. B* **2002**, *65*, 104429.

(2) Djordjevic, M.; Münzenberg, M. *Phys. Rev. B* **2007**, *75*, 012404.

(3) Carpene, E.; Mancini, E.; Dallera, C.; Brenna, M.; Puppin, E.; De Silvestri, S. *Phys. Rev. B* **2008**, *78*, 174422.

(4) Mendil, J.; Nieves, P.; Chubykalo-Fesenko, O.; Walowski, J.; Santos, T.; Pisana, S.; Münzenberg, M. *Sci. Rep.* **2014**, *4*, 3980.

(5) Jeong, T.; Zhu, J.-G.; Chung, S.; Gibbons, M. R. *J. Appl. Phys.* **2012**, *111*.

(6) Liang, W.; Schäfer, S.; Zewail, A. H. *Chem. Phys. Lett.* **2012**, *542*, 8–12.

(7) Kohn, A.; Habibi, A. *JEOL News* **2012**, *47*, 17–22.

(8) Lau, J.; Schofield, M.; Zhu, Y. *Ultramicroscopy* **2007**, *107*, 396–400.

(9) De Graef, M. *Introduction to Conventional Transmission Electron Microscopy*; Cambridge University Press, 2003.

(10) De Graef, M., Zhu, Y., Eds. *Magnetic Imaging and Its Applications to Materials*; Academic Press, 2000.

(11) Petford-Long, A. K.; De Graef, M. *Characterization of Materials*; John Wiley & Sons, Inc., 2002.

(12) Humphrey, E.; Phatak, C.; Petford-Long, A.; De Graef, M. *Ultramicroscopy* **2014**, *139*, 5–12.

(13) Volkov, V.; Zhu, Y.; De Graef, M. *Micron* **2002**, *33*, 411–416.

(14) Uhlig, T.; Rahm, M.; Dietrich, C.; Höllinger, R.; Heumann, M.; Weiss, D.; Zweck, J. *Phys. Rev. Lett.* **2005**, *95*, 237205.

(15) Chaikin, P. M.; Lubensky, T. C. *Principles of Condensed Matter Physics*; Cambridge University Press, 2000.

(16) Kosterlitz, J. M.; Thouless, D. J. *J. Phys. C: Solid State Physics* **1973**, *6*, 1181–1203.

(17) Berezinskii, V. *Sov. Phys. JETP* **1971**, *32*, 2–9.

(18) Berthier, L.; Holdsworth, P. C. W.; Sellitto, M. *J. Phys. A: Math. Gen.* **2001**, *34*, 1805–1824.

(19) Jelić, A.; Cugliandolo, L. F. *Journal of Statistical Mechanics: Theory and Experiment* **2011**, *2011*, P02032.

(20) Metropolis, N.; Rosenbluth, A. W.; Rosenbluth, M. N.; Teller, A. H.; Teller, E. *J. Chem. Phys.* **1953**, *21*, 1087–1092.
